# Supplementary material for: Flat bands and multi-state memory devices from chiral domain wall superlattices in magnetic Weyl semimetals
Source: arXiv:2303.16918 source file (2023-10-23)
Supplement: Supplementary file 1 [file supplementary2.tex]

\newcommand{\vket}[2]{
\begin{bmatrix} #1 \\ #2 \end{bmatrix}
}

\newcommand{\hbra}[2]{
\begin{bmatrix} #1  \; #2 \end{bmatrix}
}

\onecolumngrid
\appendix
\section{Supplementary information}

\subsection{Bloch wall hamiltonian spectrum with $k_{||} = 0$}
\label{suppblochgammaderivation}
First, one can choose the equivalent block-diagonal $\tau_z$ matrix for the momentum term in Eq.~\ref{eq:PWhamiltonian} and set m = 0. This decouples the left (-) and right (+) helical states $\eta$, and allows one to express the Hamiltonian of the infinitely-periodic hamiltonian with helical exchange field as follows. Let $\Omega = \frac{J}{2\hbar v_f}$, and let $G=\frac{2\pi}{a_S} = \vec{b}_x$ be the superlattice reciprocal vector. We use the definition for $\boldsymbol{\beta}(r)\boldsymbol{\beta}(r)$ in section II: 
\begin{eqnarray}
    \label{FT-exchange}
    \boldsymbol{\beta}_N(r) = J(\cos(\theta_r)\hat{y} + \sin(\theta_r)\hat{x}) = \frac{J}{2}(e^{i G x}\hat{y}+e^{-i G x}\hat{y} + -ie^{i G x}\hat{x}+ie^{-i G x}\hat{x}), \\\boldsymbol{\beta}_B(r) = J(\cos(\theta_r)\hat{y} + \sin(\theta_r)\hat{z}) = \frac{J}{2}(e^{i G x}\hat{y}+e^{-i G x}\hat{y} + -ie^{i G x}\hat{z}+ie^{-i G x}\hat{z}).
\end{eqnarray}

In Fourier space, this can be written as:
\begin{eqnarray}
    \widetilde{\boldsymbol{\beta}}^N_{G'-G} = \frac{J}{2}[(i\hat{x} + \hat{y})\delta(G'-G-\vec{b}_x) + (-i\hat{x} + \hat{y})\delta(G'-G+\vec{b}_x)]; \\
    \widetilde{\boldsymbol{\beta}}^B_{G'-G} = \frac{J}{2}[(i\hat{z} + \hat{y})\delta(G'-G-\vec{b}_x) + (-i\hat{z} + \hat{y})\delta(G'-G+\vec{b}_x)].
\end{eqnarray}

We will now focus on the Bloch wall case. 
\begin{equation}
    \hat{H}_B(k) = \hbar v_f\begin{bmatrix}
    \ddots & \Omega (\sigma_y + i \sigma_z) &    &      &    \\
     \Omega (\sigma_y - i \sigma_z) & \eta(k_x + G)\sigma_x       & \Omega (\sigma_y + i \sigma_z)   &     &    \\
      &         \Omega (\sigma_y - i \sigma_z)& \eta (k_x)\sigma_x         & \Omega (\sigma_y + i \sigma_z)    &     \\
      &         &           \Omega (\sigma_y - i \sigma_z)&     \eta (k_x - G)\sigma_x      & \Omega (\sigma_y + i \sigma_z)   \\
      &         &           &           \Omega (\sigma_y - i \sigma_z)& \ddots
  \end{bmatrix}
\end{equation}

Then, the basis transformation corresponding to a $120^{\circ}$ rotation about $\hat{x} +\hat{y} + \hat{z}$ can be used to transform the spin matrices:
\begin{eqnarray}
\sigma_y \rightarrow -\sigma_x  \nonumber \\
\sigma_z \rightarrow \sigma_y \nonumber \\
\sigma_x \rightarrow -\sigma_z \nonumber
\end{eqnarray}
and, knowing that $\sigma_+ = \sigma_x + i \sigma_y; \sigma_- = \sigma_x - i \sigma_y$, the Hamiltonian can be rewritten as:
\begin{equation}
    \hat{H}_B(k) = -\hbar v_f\begin{bmatrix}
    \ddots & 2\Omega (\sigma_-) &    &      &    \\
     2 \Omega (\sigma_+) & \eta(k_x + G)\sigma_z       & \Omega (\sigma_-)   &     &    \\
      &         2\Omega (\sigma_+)& \eta (k_x)\hat{\sigma}_z         & 2\Omega (\sigma_-)    &     \\
      &         &           2\Omega (\sigma_+)&     \eta (k_x - G)\hat{\sigma}_z      & 2\Omega (\sigma_-)   \\
      &         &           &           \Omega (\sigma_+)& \ddots
  \end{bmatrix}
\end{equation}
\begin{equation}
  = -\hbar v_f \bigoplus_n \left(\begin{bmatrix}
  -\eta(k_x + (n+1)G) & 2\Omega \\
  2\Omega & \eta(k_x + n G)
  \end{bmatrix}\right) = -\hbar v_f \bigoplus_n \left(-\eta k_x \sigma_z + 2 \Omega \sigma_x - \eta n G \sigma_z -\eta G\frac{1}{2}(\sigma_z+\sigma_0)\right)
\end{equation}

\begin{equation}
= -\hbar v_f \bigoplus_n (\icol{2\Omega \\ 0 \\ -\eta(k_x +  G (n + \frac{1}{2}))}\cdot\boldsymbol{\sigma} - \eta G \frac{1}{2}\sigma_0) = \bigoplus_n \hat{H}_n
\end{equation}
with the spectrum of $\hat{H}_n$ (thus, a diagonal subblock of $\hat{H}_B(k_{||}=\Gamma))$ given as:

\begin{equation}
    E_n = -\hbar v_f \left( \pm\sqrt{4\Omega^2 + (k_x + G(n+\frac{1}{2}))^2} - \eta G / 2\right) = \mp \sqrt{J^2 + \hbar^2 v_f^2 (k_x + \frac{\pi}{a_S}(2 n+1))^2} + \hbar v_f  \frac{\eta \pi}{a_S}
\end{equation}

\subsection{Decomposing Bloch exchange helix Hamiltonian}
First, it is useful to rotate the problem with $G=\frac{2\pi}{a_S}$ in $\hat{z}$ while preserving the Bloch magnetization $\boldsymbol{\beta}_B$'s helicity:

\begin{equation}
    \boldsymbol{\beta}_B = \text{J(cos}(G z)\hat{x} + \text{sin}(G z)\hat{y}
\end{equation}

Introducing $G^\pm = e^{\pm i G z}$ and absorbing $\hbar$ into $v_f$, we can rewrite the Hamiltonian $\hat{H}_B$ for one chirality $\eta$:

\begin{equation}
    \hat{H}_B = -i \eta v_f (\frac{\partial}{\partial x} \sigma_x + \frac{\partial}{\partial y} \sigma_y + \frac{\partial}{\partial z} \sigma_z) + J(G^+\sigma_+ + G^-\sigma_-)   
\end{equation}

We can then Fourier transform the Hamiltonian in x and y, and change the basis of $\hat{H}_B$ so as to diagonalize the helical exchange term:

\begin{align}
    \hat{H}'_B = \frac{1}{2}\begin{bmatrix}
        G^- & 1 \\
        -G^- & 1
    \end{bmatrix}
    \begin{bmatrix}
        -i \eta v_f \partial_z & \eta v_f k_x -i \eta v_f k_y + J G^+ \\
        \eta v_f k_x + i \eta v_f k_y + J G^- & i \eta v_f \partial_z \\
    \end{bmatrix} 
    \begin{bmatrix}
        G^+ & -G^+ \\
        1 & 1
    \end{bmatrix}. \\
    = \frac{1}{2}\begin{bmatrix}
        G^- & 1 \\
        -G^- & 1
    \end{bmatrix}
    \begin{bmatrix}
        A & B\\
        C & D \\
    \end{bmatrix}; \\
    A = G G^+\eta v_f - i \eta v_f G^+ \partial_z+JG^+ + \eta v_f \left(k_x-i k_y\right), \nonumber \\
    B = i \eta v_f G^+ \partial_z - G\eta v_f G^+ + JG^+ + \eta v_f \left(k_x - i k_y\right), \nonumber \\
    C = J + \eta v_f G^+\left(k_x +i k_y \right) + i \eta v_f \partial_z \nonumber, \\
    D = -J - \eta v_fG^+\left(k_x + i k_y\right) +i\eta v_f \partial_z;\nonumber \\ 
    \nonumber \\ 
    = \frac{1}{2}
    \begin{bmatrix}
        G^- A+C & G^-B+D\\
        -G^-A+C & -G^-B+D \\
    \end{bmatrix}; \\
    G^- A+C = G \eta v_f  + 2J + k_x \eta v_f \left(G^++G^-\right) + i k_y \eta v_f \left(G^+-G^-\right), \nonumber \\ 
    G^- B+D = 2 i \eta v_f \partial_z  - G \eta v_f  + k_x \eta v_f \left(-G^++G^-\right) - i k_y \eta v_f \left(G^++G^-\right), \nonumber \\ 
    -G^- A+C = - G \eta v_f  + 2 i \eta v_f \partial_z + k_x \eta v_f \left(G^+-G^-\right) + i k_y \eta v_f \left(G^++G^-\right), \nonumber \\ 
    -G^- B+D = G \eta v_f  - 2J - k_x \eta v_f \left(G^++G^-\right) - i k_y \eta v_f \left(G^+-G^-\right). \nonumber \\ 
\end{align}

Switching to cylindrical coordinates in x and y, we can define $k_x = \text{cos}(\theta_k)k_r$ and $k_y = \text{sin}(\theta_k)k_r$. We can also rewrite the above expressions: 

\begin{align}
    G^- A+C = G \eta v_f  + 2J + k_r \text{cos}(\theta_k) \eta v_f \left(G^++G^-\right) + i k_r \text{sin}(\theta_k \eta v_f \left(G^+-G^-\right), \nonumber \\ 
    G^- B+D = 2 i \eta v_f \partial_z  - G \eta v_f  + k_r \text{cos}(\theta_k) \eta v_f \left(-G^++G^-\right) - i k_r \text{sin}(\theta_k) \eta v_f \left(G^++G^-\right), \nonumber \\ 
    -G^- A+C = - G \eta v_f  + 2 i \eta v_f \partial_z + k_r \text{cos}(\theta_k) \eta v_f \left(G^+-G^-\right) + i k_r \text{sin}(\theta_k) \eta v_f \left(G^++G^-\right), \nonumber \\ 
    -G^- B+D = G \eta v_f  - 2J - k_r \text{cos}(\theta_k) \eta v_f \left(G^++G^-\right) - i k_r \text{sin}(\theta_k) \eta v_f \left(G^+-G^-\right); \nonumber \\ 
    \nonumber \\ 
    G^- A+C = G \eta v_f  + 2J + k_r \eta v_f \left( e^{i\theta_k} G^+ + e^{-i\theta_k}G^- \right), \nonumber \\ 
    G^- B+D = 2 i \eta v_f \partial_z  - G \eta v_f  +k_r \eta v_f \left(-e^{i\theta_k}G^+ + e^{-i\theta_k}G^-\right), \nonumber \\ 
    -G^- A+C = - G \eta v_f  + 2 i \eta v_f \partial_z + k_r \eta v_f \left(e^{i\theta_k}G^+ - e^{-i\theta_k}G^-\right), \nonumber \\ 
    -G^- B+D = G \eta v_f  - 2J - k_r \eta v_f \left( e^{i\theta_k} G^+ + e^{-i\theta_k}G^- \right); \nonumber \\ 
    \nonumber \\
    \hat{H}'_B=
    \begin{bmatrix}
        \frac{G \eta v_f}{2} + J + k_r \eta v_f \text{cos}(Gx + \theta_k) &  i \eta v_f \partial_z  - \frac{G \eta v_f}{2}  -i k_r \eta v_f \text{sin}(Gx + \theta_k)\\
        i \eta v_f \partial_z  - \frac{G \eta v_f}{2} + i k_r \eta v_f \text{sin}(Gx + \theta_k) & \frac{G \eta v_f}{2} - J - k_r \eta v_f \text{cos}(Gx + \theta_k) \\
    \end{bmatrix} \nonumber \\
    = \frac{G \eta v_f}{2}\hat{\sigma}_0 + \left(J+k_r\eta v_f \text{cos}(Gx + \theta_k)\right)\hat{\sigma}_z + \left(i \eta v_f \partial_z  - \frac{G \eta v_f}{2}\right)\hat{\sigma}_x +k_r\eta v_f \text{sin}(Gx + \theta_k)\hat{\sigma}_y
\end{align}

We can notice that $\hat{H}_B$ permits a continuous set of spatially translated solutions for each value of $\theta_k$. Here, we will also stop and note the correspondence with \ref{suppblochgammaderivation} for $k_r = 0$. We may also notice that a $k_r$ corresponding to the position of the uniformly-magnetized $|L\rangle$-chiral weyl node,

%\begin{align}
%    \hat{H}'_B  = \frac{G \eta v_f}{2}\hat{\sigma}_0 + \left(J+k_r\eta v_f \text{cos}(Gz + \theta_k)\right)\hat{\sigma}_z + \left(i \eta v_f \partial_z  - \frac{G \eta v_f}{2}\right)\hat{\sigma}_x +k_r\eta v_f G \text{sin}(Gz+\theta_k) \hat{\sigma}_y
% \end{align}
\begin{equation}
    k_{||} = \frac{-\eta J}{v_f},
\end{equation}
will cancel the spatially constant terms of $\hat{\sigma}_z$ using a taylor series around $\theta_k=0$ in z:
\begin{align}
    \hat{H}'_B\left(k=\frac{-\eta J}{v_f}\right)  = \frac{G \eta v_f}{2}\hat{\sigma}_0 + J\frac{\left(Gx\right)^2}{2}\hat{\sigma}_z + \left(i \eta v_f \partial_z  - \frac{G \eta v_f}{2}\right)\hat{\sigma}_x - J G x \hat{\sigma}_y.
\end{align}
Giving us the insight that the Hamiltonian is locally akin to the Dirac Hamiltonian with an additional off-diagonal term which, if the wavefunctions are represented in a hermite-gauss function basis, will generate $|n\pm2\rangle$ states. Squaring $\left(H'_B-\eta \hbar v_f G/2\right)$ at this $k_{||}$ allows us to nearly decouple the Hamiltonian for each exchange eigenspinor, giving an insight on the form of the wavefunctions as discussed in the main text:

\begin{align}
    \left(H'_B-\eta \hbar v_f G/2\right)^2 = \eta \hbar v_f G J \left[\text{sin}(Gz+\theta_k)\hat{\sigma}_y -  \text{cos}(Gz+\theta_k)\hat{\sigma}_z\right] \nonumber \\ +\left[\left(\frac{\hbar v_f G}{2}\right)^2 -\hbar^2 v_f^2 \left(\partial_z^2 +i G \partial_x\right) + 2J^2\left(1-\text{cos}(Gz+\theta_k)\right)\right]\hat{\sigma}_0.
\end{align}

We are unable to solve this exactly, but can manipulate the spin terms of $\left(H_B-E\right)|\Psi\rangle = 0$ to generate constraints on the wavefunctions, defining $\Lambda = \left(\eta k_{||} e^{i \theta_{k}} +Je^{-iGx} \right)^{-1}$.
\begin{align}
    \left[\left(\hbar v_f\right)^2 \left(\Lambda^+ \partial_x^2 + \frac{\partial \Lambda^+}{\partial x}\partial_x \right) +i\eta \hbar v_f \frac{\partial \Lambda^+}{\partial x}E - \Lambda^+ E^2+ \frac{1}{\Lambda}\right]|\uparrow\rangle = 0, \\ 
    \left[\left(\hbar v_f\right)^2 \left(\Lambda \partial_x^2 + \frac{\partial \Lambda}{\partial x}\partial_x \right) -i\eta \hbar v_f \frac{\partial \Lambda}{\partial x}E - \Lambda E^2+ \frac{1}{\Lambda^+}\right]|\downarrow\rangle  = 0,\label{downbloch}\\
    |\downarrow\rangle = -\Lambda^+ \left(-i\eta v_f \partial_z - E\right)|\uparrow\rangle,\\
    |\uparrow\rangle = -\Lambda \left(i\eta v_f \partial_z - E\right)|\downarrow\rangle. \label{upbloch}
\end{align}

 Composing Eq. \ref{downbloch} and Eq. \ref{upbloch} at $k_{||} = \frac{-\eta J}{\hbar v_f}$ and $E = \eta \hbar v_f G/4$, we can find two solutions for a $|\Psi\rangle$ with normalization coefficients $\mathbb{C}_1, \mathbb{C}_2$:

 \begin{align}
     |\Psi\rangle = \frac{1}{{\sqrt[4]{e^{i G x}}}}\left[\mathbb{C}_1 e^{\frac{2 J \left(1+e^{i G x}\right)}{G \hbar v_f \sqrt{e^{i G x}}}}+\mathbb{C}_2 e^{-\frac{2 J \left(1+e^{i G x}\right)}{G \hbar v_f \sqrt{e^{i G x}}}}\right]|\downarrow\rangle \nonumber \\
     -\frac{1}{e^{i G x}-1}\left[\eta  \sqrt[4]{e^{i G x}} \left(-1+e^{i G x}\right) e^{-\frac{2 J \left(1+e^{i G x}\right)}{G \hbar v_f \sqrt{e^{i G x}}}} \left(\mathbb{C}_1 e^{\frac{4 J \left(1+e^{i G x}\right)}{G \hbar v_f \sqrt{e^{i G x}}}}-\mathbb{C}_2\right)\right]|\uparrow\rangle.
 \end{align}

A similar solution should likely hold true for the two other expressions. 

\begin{align}
    H_B^2 = J^2\frac{\left(Gz\right)^4}{4} \hat{\sigma}_0 + J\frac{\left(Gz\right)^2}{2} v_f \eta \left(i\partial_x - \frac{G}{2}\right)i\hat{\sigma}_y - J\frac{\left(Gz\right)^2}{2} v_f \eta \left(i\partial_x - \frac{G}{2}\right)i\hat{\sigma}_y - J\frac{\left(Gz\right)^3}{2} i \hat{\sigma}_x + J\frac{\left(Gz\right)^3}{2} i \hat{\sigma}_x \nonumber \\
    - v_f \eta J G^2 z \hat{\sigma}_z + v_f^2\left(-\partial_z^2 -iG\partial_z +\frac{G}{4}\right)\hat{\sigma}_0 + \eta v_f J G z\left(i\partial_z - \frac{G}{2} \right)i\hat{\sigma_z} - \eta v_f J G z\left(i\partial_z - \frac{G}{2} \right)i\hat{\sigma_z} + J^2 \left(Gz\right)^2\hat{\sigma}_0 \nonumber \\ \nonumber \\
    = J^2\frac{\left(Gz\right)^4}{4} \hat{\sigma}_0  - v_f \eta J G^2 z \hat{\sigma}_z + v_f^2\left(-\partial_z^2 -iG\partial_z +\frac{G}{4}\right)\hat{\sigma}_0 + J^2 \left(Gz\right)^2\hat{\sigma}_0.
\end{align}

Dropping the quartic term, letting $s=\pm1$ denote the $\pm J$ eigenvalue exchange eigenspinor, and changing the superlattice direction back to x as in the main text, we can write out $H_B^2$ as thus:

\begin{equation}
    H_{B,s}^2 = v_f^2\left(-\partial_x^2 - i G\partial_x +\frac{G^2}{4}\right) + J\left(Gx\right)^2 -sv_f\eta J G\left(Gx +1\right)\hat{\sigma}_z + 
\end{equation}

Unfortunately, this does not permit elegant harmonic oscillator wavefunctions as we may hope; the $-iG\partial_z$ and $v_fJG^2x$ terms are of the same order of magnitude as the parabolic potential and $\hat{p}^2_x$ operator. Despite this, the Wolfram Mathematica software does provide two solutions for the null space of $\left(\hat{H}_B^2 -E^2\right)$ in terms of the generalized nth ($n\in \mathbb{R}$) Hermite polynomial $H_n(x)$ and the Kummer confluent hypergeometric function $_{1}F_{1}$:

\begin{align}
        |s,1\rangle = e^{\frac{G}{2}\left(-ix + \eta s x - \frac{Jx^2}{v_f}\right)} H_n\left(-\eta s \sqrt{\frac{G v_f}{4J}}+x\sqrt{\frac{GJ}{v_f}}\right), \\
        |s,2\rangle = e^{\frac{G}{2}\left(-ix + \eta s x - \frac{Jx^2}{v_f}\right)}{}_{1}F_1\left(\frac{-n}{2};\frac{1}{2};\left(-\eta s \sqrt{\frac{G v_f}{4J}}+x\sqrt{\frac{GJ}{v_f}}\right)^2\right),
\end{align}

Where $n$ is
\begin{equation}
    n = \frac{\left(4E^2 -4 G J v_f + 4 \eta G J s v_f + G^2v_f^2 \right)}{8GJv_f}.
\end{equation}

\subsection{Landau level picture of Bloch exchange helix}

First, it is useful to rotate the problem with $G=\frac{2\pi}{a_S}$ in $\hat{z}$ while preserving the Bloch magnetization $\boldsymbol{\beta}_B$'s helicity:

\begin{equation}
    \boldsymbol{\beta}_B = \text{J(cos}(G z)\hat{x} + \text{sin}(G z)\hat{y}
\end{equation}

Introducing $G^\pm = e^{\pm i G z}$ and letting $\hbar=1$ we can rewrite the Hamiltonian $\hat{H}_B$ for one chirality $\eta$:

\begin{equation}
    \hat{H}_B = -i \eta v_f (\frac{\partial}{\partial x} \sigma_x + \frac{\partial}{\partial y} \sigma_y + \frac{\partial}{\partial z} \sigma_z) + J(G^+\sigma_+ + G^-\sigma_-)   
\end{equation}

We can then choose a basis to expand our solutions $|s,n,\mathbf{k}\rangle$ in. We observe that the bands are dispersive in $\hat{x}$ and $\hat{y}$, and since we know the pseudomagnetic length $l_B = \sqrt{\frac{\hbar}{e |\mathbf{B}^5|}} = \sqrt{\frac{\hbar v_f a_S }{2 \pi J}} \approx \text{8 nm} >> a_0 \approx 1$ nm, with $l_B << a_S \approx 100$ nm; we choose to use the harmonic oscillator eigenfunctions $|n, \mu_z\rangle$ centered around a point $\mu_z$ in $\hat{z}$. 

\begin{equation}
\Psi_{n,\mu_z} (z) = \langle z | n, \mu_z\rangle = H_n\left(\frac{z-\mu_z}{l_B}\right)\frac{1}{\sqrt{2^n n! \sqrt{\pi} \, l_B}}e^{\frac{-(z-\mu_z)^2}{2 l_B^2}} 
\end{equation}

with useful properties
\begin{eqnarray}
 \label{xop} z|n\rangle = \frac{l_B}{\sqrt{2}}\left(\sqrt{n}|n-1\rangle + \sqrt{n+1}|n+1\rangle\right) \\
\frac{\partial}{\partial z} |n\rangle = \frac{1}{l_B\sqrt{2}}\left(\sqrt{n}|n-1\rangle - |n+1\rangle \right)
\end{eqnarray}

For the spin component, we note that

\begin{equation}
    |s,n, \mu_z \rangle = \frac{1}{\sqrt{2}}\vket{s e^{i G z}}{1}\otimes|n, \mu_z \rangle
\end{equation}

are eigenfunctions of $J \boldsymbol{\beta}_B\cdot\boldsymbol{\sigma}$, which we can be shown from Eq.~\ref{Jbetasigmaeig}. Using an intuition about landau levels (that the states will be localized in the directions orthogonal to $B_5$), and knowing that the landau level basis states will decay on a scale much smaller than the superlattice, thus allowing phase slips between states in z with minimal contribution to the $\hat{p}_z$ term, we will make a guess for such a wavefunction localized near a point $z = \mu_z$. For this, it is also useful to define a sawtooth waveform:

\begin{eqnarray}
\text{saw}(z)=\text{mod}(z-\frac{a_s}{2},a_s) - \frac{a_s}{2}; \\
|\Psi_{s,n,\mu_z} (\mathbf{k})\rangle = e^{i \mathbf{k}\cdot\mathbf{R}}e^{-i\left(cos(G\mu_z)k_y y+sin(G\mu_z)k_x x + k_z \text{saw}(z-\mu_z)\right)}|s,n,\mu_z\rangle 
\end{eqnarray}

Probing around $\mu_z = 0$, we recover the expected wavefunction which, after a basis transform in spin space, can be made to only disperse in $k_x$. This is explicitly shown below for the $| \downarrow\,\rangle $ spin component:

\begin{eqnarray}
\label{ansatz} |\Psi_{s,n,\mu_z} (\mathbf{k})\rangle 
= e^{i k_x x + 0 + ik_z (z - \text{saw}(z))}|s,n, \mu_z=0\rangle \approx e^{i k_x x } \frac{1}{\sqrt{2}}\vket{s e^{iGz}}{1} |n, \mu_z =0\rangle. 
\end{eqnarray}

We can also show that these states at different $\mu_z$ are orthogonal:

\begin{eqnarray}
\langle \Psi_{s',n',\mu_z'} (\mathbf{k}) | \Psi_{s,n,\mu_z } (\mathbf{k}) \rangle = e^{ik_z 0}\int e^{i(cos(G\mu_z')k_y y - cos(G\mu_z)k_y y} dy \, \int e^{i(sin(G\mu_z')k_x x - sin(G\mu_z)k_x x} dx \,\langle s', n'_{\mu_z'}| s, n_{\mu_z} \rangle  \nonumber \\
= \delta(cos(G\mu_z')-cos(G\mu_z))\,\delta(sin(G\mu_z')-sin(G\mu_z)) \,\langle s', n'_{\mu_z'}| s, n_{\mu_z} \rangle  = \delta(\text{mod}(\mu_z' - \mu_z, \frac{2\pi}{G})) \langle s', n'_{\mu_z'}| s, n_{\mu_z} \rangle \nonumber \\ 
\approx \delta(\mu_z' - \mu_z) \langle s', n'| s, n\rangle = \delta(\mu_z' - \mu_z) \delta(s'-s) \delta(n'-n) 
\end{eqnarray}

Factoring out the envelope function and instead considering a linear combination of these states in z, we can write the full ansatz Hamiltonian eigenfunctions, fulfilling Bloch's theorem, as:

\begin{equation} \label{fullblochfunct}
    |s,n,\mathbf{k}\rangle = e^{i\mathbf{k}\cdot\mathbf{R}} \int_{-\infty}^{\infty}e^{-i(cos(G \mu_z)k_y y+sin(G \mu_z)k_x x + k_z\text{saw}(z-\mu_z)}|s,n, \mu_z\rangle \, d\mu_z  
\end{equation}

Since the states in $\mu_z$ are orthogonal with degenerate spectrum, we can write a new wavefunction with $\mu_z$ quantum number:

\begin{eqnarray}
    |s,n,\mathbf{k}\rangle = \int_{0}^{a_s} |s,n,\mu_z,\mathbf{k}\rangle \; d\mu_z \\
    |s,n,\mu_z,\mathbf{k}\rangle = \sum_{m=-\infty}^{\infty} |\Psi_{s,n,\mu+m a_s} (\mathbf{k})\rangle = e^{i \mathbf{k} \cdot \mathbf{R}}\text{U}_{s,n,\mu_z}(\mathbf{R})  
\end{eqnarray}

We will henceforth let $|s,n,\mathbf{k}\rangle$ only refer to a single $|s, \, n,\, \mu_z=0,\, \mathbf{k}\rangle$ in Eq.~\ref{ansatz}, recovering the spectrum from symmetry arguments. For the $z |n\rangle $ and $\partial_z |n\rangle$ terms, we will also exploit the discrete translation symmetry of the Hamiltonian to say $\langle \Psi_{s',n',0} (\mathbf{k})|\hat{O}|\Psi_{s',n',0} (\mathbf{k})\rangle = \langle s', \, n',\, 0,\, \mathbf{k}|\hat{O}|s, \, n,\,0,\, \mathbf{k}\rangle $, though this will break for $\partial_z \left(e^{-ik_z \text{saw}(k_z)}\right)$ and will be treated on its own (Eq.~\ref{saw}). It is also useful to make note of the approximations $\text{sin}(Gz)\approx Gz$ and $\text{cos}(Gz)\approx1$ to first order, and will also define the $\tau$ matrices in s space. We can then project these states onto the Hamiltonian:

\begin{eqnarray}
    \langle s', n', \mathbf{k}|\hat{H}_B| s, n, \mathbf{k}\rangle = -i \eta v_f \langle s', n', \mathbf{k}|\frac{\partial}{\partial x} \sigma_x | s, n, \mathbf{k}\rangle + -i \eta v_f \langle s', n', \mathbf{k}|\frac{\partial}{\partial y} \sigma_y | s, n, \mathbf{k}\rangle \nonumber \\ -i \eta v_f \langle s', n', \mathbf{k}|\frac{\partial}{\partial z} \sigma_z | s, n, \mathbf{k}\rangle +  
    J \langle s', n', \mathbf{k}| \boldsymbol{\beta}_B\cdot\boldsymbol{\sigma} | s, n, \mathbf{k}\rangle; \\ \nonumber \\
    \label{ddxsx} -i \eta v_f \langle s', n', \mathbf{k}|\frac{\partial}{\partial x} \sigma_x | s, n, \mathbf{k}\rangle = \frac{\eta v_f k_x}{2}\langle n' |\hbra{s'G^-}{1}\vket{1}{sG^+}|n\rangle =  \eta v_f k_x \begin{cases}
          s \langle n'| cos(Gz) |n \rangle   \quad &\text{if} \, s' = s \\
          -i s \langle n'| sin(Gz) |n \rangle \quad &\text{if} \, s' = -s \\
     \end{cases}  \nonumber \\ 
     \approx \eta v_f k_x s \delta(s'-s) \delta(n'-n) -i \eta v_f k_x s \delta(s'+s) \langle n'|G l_B\left(\sqrt{\frac{n}{2}}|n-1\rangle + \sqrt{\frac{n+1}{2}}|n+1\rangle\right) \nonumber \\ 
     = \eta v_f k_x\left(\tau_z\delta(n'-n) + G l_B \tau_y\left[\sqrt{\frac{n}{2}}\delta(n'-n+1) + \sqrt{\frac{n+1}{2}}\delta(n'-n-1)\right]\right) \\ \nonumber \\
     \label{ddysy} -i \eta v_f \langle s', n', \mathbf{k}|\frac{\partial}{\partial y} \sigma_y | s, n, \mathbf{k}\rangle =  \langle n' |\hbra{s'G^-}{1}0\vket{i}{-isG^+}|n\rangle = 0 \\
     -i \eta v_f \langle s', n', \mathbf{k}|\frac{\partial}{\partial z} \sigma_z | s, n, \mathbf{k}\rangle = \frac{-i \eta v_f}{2}\langle n' |\hbra{s'G^-}{1} \partial_z (\vket{sG^+}{-1}|n\rangle) + \eta v_f\Xi =  \nonumber \\
     \frac{-i\eta v_f}{2}\langle n'|\hbra{s'G^-}{1}\left(\vket{siGG^+}{0}|n\rangle + \vket{sG^+}{-1}(\frac{\sqrt{\frac{n}{2}}}{l_B}|n-1\rangle - \frac{\sqrt{\frac{n+1}{2}}}{l_B}|n+1\rangle)\right) + \eta v_f \Xi \nonumber \\ 
     = \frac{\eta v_f}{2} G s's\,\delta(n'-n) - \frac{\eta v_f k_z}{2}\xi_{n',n}(s's-1)  + \frac{-i\eta v_f}{2 l_B}(s's-1)\sqrt{\frac{n}{2}}\delta(n'-n+1) - \sqrt{\frac{n+1}{2}}\delta(n'-n-1)\nonumber \\
     = \frac{\eta v_f G}{2} (\tau_0 - \tau_x) \,\delta(n'-n) + \eta v_f k_z \tau_x \xi_{n',n}+ \frac{i\eta v_f}{ l_B}\tau_x\left[\sqrt{\frac{n}{2}}\delta(n'-n+1) - \sqrt{\frac{n+1}{2}}\delta(n'-n-1)\right] \\ \nonumber \\
     J \langle s', n', \mathbf{k}| \boldsymbol{\beta}_B\cdot\boldsymbol{\sigma} | s, n, \mathbf{k}\rangle = \frac{J}{2} \langle n'| \hbra{s'G^-}{1}(G^+\sigma_+ +G^-\sigma_-)\vket{sG^+}{1}|n\rangle = J \langle n'| \hbra{s'G^-}{1}\vket{G^+}{s}|n\rangle \label{Jbetasigmaeig}\nonumber \\
     = \frac{J}{2} (s'+s)\langle n'|n\rangle = J \tau_z\delta(n'-n)
\end{eqnarray}

We will also step through and further scrutinize that which is relevant to $\Xi$ and $\xi_{n',n}$, i.e. concerning the term in the product rule expansion that is generated by phase slips in z. 

\begin{eqnarray} \label{saw}
\Xi_{n',n} = \frac{i}{2} \sum_{m=-\infty}^{\infty}(\langle n'_{0+m a_s}|)\hbra{s'G^-}{1} e^{ik_z (\text{saw}(z) - z) } \partial_z (e^{-i k_z\, (\text{saw}(z) - z)}) \vket{sG^+}{-1}\sum_{m=-\infty}^{\infty}(|n_{0+m a_s}\rangle) \nonumber \\
=i \frac{s's-1}{2} \sum_{m=-\infty}^{\infty}(\langle n'_{0+m a_s}|) \; \sum_{m=-\infty}^{\infty} i k_z \delta(x-\frac{a_S}{2}+m a_S)\sum_{m=-\infty}^{\infty}(|n_{0+m a_s}\rangle)dz
\end{eqnarray}

This can be motivated by viewing the $\text{saw}(z)-z$ function as a linear combination of shifted Heaviside step functions, the differentiation of which generates a Dirac comb with the period of the lattice. Integrating only over one lattice period, being that we are taking the inner product of the lattice-periodic part of the Bloch function, and neglecting the landau basis states with $m\neq 0, 1$, we can rewrite the above expression as:

\begin{eqnarray}
\Xi_{n',n} \approx - k_z \frac{s's-1}{2} \int_{0}^{a_0} ( \Psi_{n',0}^*(x) + \Psi_{n',a_S}^*(x))\delta(x-\frac{a_S}{2})(\Psi_{n,0}(x) + \Psi_{n,a_S}(x)) \, dz \nonumber \\
=  - k_z \frac{s's-1}{2} \left( \Psi^*_{n,0}(\frac{a_s}{2}) + \Psi^*_{n,a_S}(\frac{a_s}{2})\right)\left(\Psi_{n,0}(\frac{a_s}{2}) + \Psi_{n,a_S}(\frac{a_s}{2})\right)\nonumber \\
\equiv  k_z \tau_x \left( \Psi_{n',0}(\frac{a_s}{2}) +\Psi_{n',0}(\frac{-a_s}{2})\right)\left(\Psi_{n,0}(\frac{a_s}{2}) + \Psi_{n,0}(\frac{-a_s}{2})\right)
\end{eqnarray}

Further simplifying, we can employ the identity $H_n(-x) = (-1)^n H_n(x)$:

\begin{equation}
\Xi_{n',n} = k_z \tau_x \begin{cases} 4 \Psi_{n'}\left(\frac{a_S}{2}\right)  \Psi_{n}\left(\frac{a_S}{2}\right) \quad &\text{if} \; \text{n' and n even} \\ 0 \quad &\text{else}  \end{cases}
\end{equation}

In the limit of z far from $\mu_z = 0$, which is true for $\sqrt{\langle x^2 \rangle } = \sqrt{\frac{2n+1}{2}}l_B = \sqrt{\frac{2n+1}{2}} \times \text{ 8 nm}  << \frac{a_S}{2} =  50$ nm in our system (thus, $n<<38$), the highest-power Hermite polynomial term will tend to dominate: 
\begin{eqnarray}
\Psi_n(z) \approx \left(\frac{2z}{l_B}\right)^n \frac{1}{\sqrt{2^n n! \sqrt{\pi} l_B}} e^{\frac{-z^2}{2 l_B^2}} \nonumber \\
= \frac{1}{\sqrt{n! \sqrt{\pi} l_B}} \left(\frac{\sqrt{2}z}{l_B}\right)^n e^{\frac{-z^2}{2 l_B^2}}
\end{eqnarray}

Thus,
\begin{equation}
\Xi_{n',n} = \eta v_f k_z \tau_x \xi_{n',n} = \eta v_f k_z \tau_x \frac{4}{\sqrt{n'! n! \pi}l_B} \left(\frac{a_S}{\sqrt{2} l_B}\right)^{n'+n} \text{exp}\left(-\frac{a^2}{4 l_B^2}\right) \delta_{n',n\in 2\mathbb{Z}} 
\end{equation}

Which we expect to be very small, and zero for most values of m, n. We will revisit it later when evaluating band flatness, but for now will neglect any off-diagonal $\xi_{n',n}$. Let us now collect the relevant terms $\mathbf{A}$ and $\mathbf{B}$ of $(\boldsymbol{A}\cdot\boldsymbol{\tau})\otimes \hat{I}_n$ and $(\boldsymbol{B}\cdot\boldsymbol{\tau})\otimes \frac{\hat{a}}{\sqrt{2}}$, defining $\boldsymbol{\tau}=\begin{bmatrix} \tau_0 & \tau_x & \tau_y & \tau_z \end{bmatrix}^T$, and rewrite $H_B(\mathbf{k})$ in the $|n\rangle\otimes|s\rangle$ basis:

\begin{eqnarray}
    \mathbf{A} = \eta v_f \begin{bmatrix}
   \frac{G}{2} \\
   k_z \xi_{n} - \frac{G}{2} \\
   0\\
   \frac{J}{\eta v_f} + k_x\\
  \end{bmatrix}; \;\; \mathbf{B} = \eta v_f \begin{bmatrix}
   0 \\
   \frac{i}{l_B} \\
   k_x G l_B\\
   0\\
  \end{bmatrix};
\end{eqnarray}

\begin{equation}
    \hat{H}_B(k) = \begin{bmatrix}
    \ddots & \sqrt{\frac{3}{2}} \mathbf{B}^*\cdot\boldsymbol{\tau} &    &      &    \\
     \sqrt{\frac{3}{2}} \mathbf{B}\cdot\boldsymbol{\tau}& \mathbf{A}\cdot\boldsymbol{\tau}       & \sqrt{\frac{2}{2}}\mathbf{B}^*\cdot\boldsymbol{\tau}   &     &    \\
      &         \sqrt{\frac{2}{2}}\mathbf{B}\cdot\boldsymbol{\tau}& \mathbf{A}\cdot\boldsymbol{\tau}         & \sqrt{\frac{1}{2}}\mathbf{B}^*\cdot\tau    &     \\
      &         &           \sqrt{\frac{1}{2}}\mathbf{B}\cdot\tau &    \mathbf{A}\cdot\boldsymbol{\tau}     
  \end{bmatrix}
\end{equation}

Let us then change the basis of $\mathbf{A,B}$ with the goal of manipulating the lower and upper diagonals into the form $\tau_-$ and $\tau_+$, respectively.

\begin{eqnarray}
\hat{S} = \begin{bmatrix}
            1 & 0 & 0 & 0 \\
            0 & 0 & 1 & 0 \\
            0 & -1 & 0 & 0 \\
            0 & 0 & 0 & 1 
            \end{bmatrix}; \;
            (\hat{S} \mathbf{B})\cdot \boldsymbol{\tau} = \eta v_f G k_x l_B \tau_x - \frac{i\eta v_f }{l_B}\tau_y \label{taumin}
\end{eqnarray}

For $\boldsymbol{B\cdot\tau} \propto \tau_- = \tau_x - i\tau_y$, then
\begin{equation}
G k_x l_B = \frac{-1}{l_B}
\end{equation}

Rearranging, recovering $\hbar$, and substituting $k_r$ for $|k_x|$, we can solve for the radial k which will allow for the construction of landau levels:

\begin{eqnarray}
k_x  = - \frac{a_S}{2 \pi l_B^2} = -\frac{a_S e \, \eta |B_5|}{2 \pi \hbar} = -\frac{\eta J}{\hbar v_f}; \\
k_r = |k_x| = \frac{J}{\hbar v_f}
\end{eqnarray};

Recovering the expected $k_r$ which gives the position of the Weyl nodes and explaining the numerical formation of landau levels. We also note here, that the Taylor series approximation used in Eq.~\ref{ddxsx} could fail when $l_B$ becomes a significant fraction of the lattice, or for higher landau levels with greater area, generating higher order creation and annihilation terms. Plugging in $l_B$, employing Eq.~\ref{taumin} and its hermitian conjugate, and applying $\hat{S}\mathbf{A}$ we can express \textcolor{red}{at least an isospectral} Hamiltonian more succinctly:

\textcolor{red}{I insert a spurious $\sqrt{2}$ here. It should be there somewhere, but I am not sure how to recover it...}

\begin{eqnarray}
    \hbar\omega_c = \frac{\eta v_f}{l_B} = \eta \sqrt{\frac{2 J h v_f}{a_s}}; \\
    \hat{H}_B(k_x = \frac{-J}{\hbar v_f }) = \hbar \omega_c \frac{\hat{a}}{\sqrt{2}} \tau_- + \hbar \omega_c \frac{\hat{a^+}}{\sqrt{2}} \tau_+ + \mathbf{A}\cdot\boldsymbol{\tau} \nonumber \\
    = \frac{\hbar \omega_c}{\sqrt{2}}\left(a\tau_- + a^+\tau_+\right)  + \frac{\eta G v_f}{2}\tau_0  + \eta v_f \frac{G- \xi_n 2k_z }{2}\tau_y + (\eta v_f \frac{- \eta J}{v_f} + J) \tau_z. \nonumber 
\end{eqnarray}

Cancelling the $\tau_z$ term, relying on $\eta^2 = 1$, we get: 
\begin{eqnarray}
   \hat{H}_B(k_z, |k_r|=k_0) = \eta
          \frac{v_f G}{2}\tau_0 + \frac{\hbar \omega_c}{\sqrt{2}}(a\tau_- + a^+\tau_+) + v_f \left( \frac{G}{2} -\xi_n k_z  \right)\tau_y \nonumber \\
\end{eqnarray}

\begin{equation}
 = \frac{\eta\hbar}{2} \begin{bmatrix}
            v_f G & \sqrt{2}\omega_c \hat{a}^+ +i v_f\left(G-2\xi_n k_z\right) \\
            \sqrt{2}\omega_c \hat{a} -i v_f\left(G-2\xi_n k_z\right) & v_f G 
            \end{bmatrix} \nonumber \\
= \hbar \omega_c \begin{bmatrix} 0 & b^+ \\ 
                                b & 0 \\ 
                \end{bmatrix} + \frac{\eta \hbar v_f G}{2}\tau_0  
\end{equation}

with spectrum: 
\begin{equation}
E_n = \frac{\eta \hbar v_f G}{2} + \text{sgn}(n) \hbar \omega_c \sqrt{n} 
\end{equation}

Recovering the observed energy spacing above the Weyl points. We can also solve for the ground-state wavefunction on one site in $\tau$ space: 

\begin{eqnarray}
\hat{b}\, \phi(x) = 0 \\
\hat{a} \phi (x) = \frac{i v_f (G - 2 \xi_n k_z)}{\sqrt{2}\omega_c } \phi (x) \\ 
= \sum_{n=0}^\infty c_n \sqrt{n} |n-1\rangle = \frac{i v_f (G - 2 \xi_n k_z)}{\sqrt{2}\omega_c } \sum_{n=0}^\infty c_n |n\rangle \\ 
= \sum_{n=0}^\infty c_{n+1} \sqrt{n+1} |n\rangle = \frac{i v_f (G - 2 \xi_n k_z)}{\sqrt{2}\omega_c } \sum_{n=0}^\infty c_n |n\rangle \\
\implies c_{n+1} = \frac{\Omega}{\sqrt{n+1} } c_n
\end{eqnarray}

Using Wolfram Mathematica, this first-order non-homogeneous recurrence relation with variable coefficients has solution 

\begin{equation}
c_n = \frac{\Omega^{n-1}}{\sqrt{\Gamma(n+1)}} = \left(\frac{i v_f (G - 2 \xi_n k_z)}{\sqrt{2}\omega_c }\right)^{n-1}\frac{1}{\sqrt{\Gamma(n+1)}}
\end{equation}

Blah blah.... What else needs to be done? Can write out the explicit wavefunctions after this. 

\begin{figure}
\centering
 \includegraphics[width = \linewidth]{supplementary_figures/blochLLs.png}
 \caption{Band structure which poorly shows the correspondence with dirac LL spacing. A better band structure plot might be chosen. I promise that they do have this spacing, but I have lost my nice plot which shows this.}
\end{figure}

\textcolor{red}{Great! Now I probably need to make some plots and corroborate this with the numerical model. It is probably also worth revisiting the thing I did with $\zeta$ to evaluate band flatness in the direction of the superlattice. }

\subsection{Landau level picture of Ne\'el exchange helix}

First, the exchange term of the Ne\'el Hamiltonian $\hat{H}_N$ can be translated in space:

\begin{equation}
    \boldsymbol{\beta}_N = J\left(\text{sin}(G x)\hat{y} - \text{cos}(G x)\hat{x}\right)
\end{equation}

giving rise to an axial magnetic field

\begin{equation}
    \mathbf{B}^5_N = \frac{2 \pi J}{a_S e v_f} \, \text{cos}(G x)
\end{equation}

with spatially-dependent axial magnetic length: 

\begin{equation}
    l_B(x) = \sqrt{\frac{\hbar}{e |\mathbf{B}^5|}} = \sqrt{\frac{\hbar v_f a_S}{2 \pi J |\text{cos}(Gx)|}} = \sqrt{\frac{|\text{sec}(G x)|}{G \Delta k}} =  l_{B_0} \sqrt{|\text{sec}(G x)|}
\end{equation}

Using the definitions described for $\hat{H}_B$, we can rewrite $\hat{H}_N$:

\begin{equation}
    \hat{H}_N = -i \eta v_f (\frac{\partial}{\partial x} \sigma_x + \frac{\partial}{\partial y} \sigma_y + \frac{\partial}{\partial z} \sigma_z) - J(G^+\sigma_- + G^-\sigma_+)   
\end{equation}

Then, we will take ansatz wavefunctions of the form

\begin{eqnarray}
    |n \rangle = \sqrt{\frac{|\text{cos}(G x)|}{2 \, l_{B_0}}}\Psi_{n}\left(\frac{\text{sin}(G x)}{G\, l_{B_0}}\right)\\ 
    |s, n\rangle = \frac{1}{\sqrt{2}}\vket{s e^{-iGx}}{-1} \otimes |n\rangle \\
    |s,n,\mathbf{k}\rangle = e^{i \mathbf{k \cdot R}} e^{-i\,\text{saw}(k_x) x} |s, n_x, n_y\rangle
\end{eqnarray}

Where a new saw() function is defined with twice the periodicity

\begin{equation}
    \text{saw}(x)=\text{mod}(x-\frac{a_s}{4},\frac{a_s}{2}) - \frac{a_s}{4},  
\end{equation}

and the Hermite-Gauss harmonic oscillator eigenfunctions are defined as usual:

\begin{equation}
    \Psi (u) = H_n\left(u\right)\frac{1}{\sqrt{2^n n! \sqrt{\pi}}}e^{\frac{-u^2}{2}}.
\end{equation}

This recovers both intuitive and numerically observed results: wavefunctions are localized in the superlattice direction around points of maximal $\mathbf{B}^5$, behaving locally like landau levels ($\frac{\text{sin}(Gx)}{G}\approx x $) and decaying with $e^{-\frac{x^2}{2l_B^2}}$ near the $\text{sin}(x) = 0$ crossings. The tanh term will cancel the $k_y$-dependence for $k_y < k_0$, flattening bands in y for momenta smaller than the Weyl cone splitting. This definition of the lattice-periodic portion of the Bloch function will allow for the generation of construction of higher and lower ladder operator states upon projection onto the Hamiltonian.

One useful property of this periodic landau level eigenbasis is, to good approximation, its orthogonality, which we can show:

\begin{eqnarray}
    \langle s', n' |s, n \rangle = \frac{1}{2} \int_0^{a_s} 
 \Psi_{n'}\left(\frac{\text{sin}(G x)}{G l_{B_0}}\right) \hbra{s' e^{i G x}}{-1}\vket{s e^{-i G x}}{-1} \Psi_n\left(\frac{\text{sin}(G x)}{G l_{B_0}}\right) |\text{cos}(Gx)| \,dx \nonumber 
\end{eqnarray}

Exploiting the symmetry of the integral, we can simplify and perform u-substitution, defining $\zeta = (G l_{B_0})^{-1} = \sqrt{\frac{a_s J}{h v_f}}$

\begin{eqnarray}
\langle s', n' |s, n \rangle =  \delta_{s',s} 2 \int_0^{a_s/4} 
 \Psi^*_{n'}\left(\frac{\text{sin}(G x)}{G l_{B_0}}\right)  \Psi_n\left(\frac{\text{sin}(G x)}{G l_{B_0}}\right) \frac{|\text{cos}(Gx)|}{l_{B_0}} \; dx \nonumber \\
 u = \frac{\text{sin}(G x)}{G l_{B_0}}; \;\;  du = \frac{\text{cos}(G x)}{l_{B_0}}\, dx \nonumber  \\
 \langle s', n' |s, n \rangle =  \delta_{s',s} \int_{-\zeta}^{\zeta} 
 \Psi^*_{n'}\left(u\right)  \Psi_n\left(u\right) du  \approx \delta_{s',s} \delta_{n',n}.
\end{eqnarray}

for $\zeta \rightarrow \infty$, this is exact. In Fig.~\ref{numorthogonality} we can numerically show that this approximation holds well for small n, and allows us to construct  an orthonormal basis. Furthermore, we can define a set of ladder operators operating on these basis states:

\begin{eqnarray}
    \hat{\chi} = \frac{\text{sin}(Gx)}{G l_{B_0}}; \\
    \hat{\rho} = -i l_{B_0} \text{sec}(Gx) \frac{\partial}{\partial x} + i \frac{G l_{B_0}}{2}\text{sec}(Gx)\text{sin}(Gx);\\
    \hat{a} = \frac{1}{\sqrt{2}}\left(\hat{\chi} + i \hat{\rho}\right)\\
    \hat{a}^+ = \frac{1}{\sqrt{2}}\left(\hat{\chi} - i \hat{\rho}\right)
\end{eqnarray}

We can show the standard commutation relation: 

\begin{eqnarray}
    [\hat{a},\hat{a}^+] = \frac{1}{2}\left(\hat{\chi}^2 + \hat{\rho}^2 -i[\hat{\chi},\hat{\rho}] - \left(\hat{\chi}^2 + \hat{\rho}^2 +i[\hat{\chi},\hat{\rho}]\right)\right) \nonumber \\
    = -i[\hat{\chi},\hat{\rho}]; \nonumber \\
    \left[\hat{\chi},\hat{\rho}\right]\psi = \frac{-i \text{sin}(Gx)}{G} \text{sec}(Gx) \frac{\partial}{\partial x} \psi + \frac{i}{2} \text{sin}^2(Gx)\text{sec}(Gx)\psi \nonumber \\
    + \frac{i}{G} \text{sec}(Gx) \frac{\partial}{\partial x} \left(\text{sin}(Gx) \psi\right) -\frac{i}{2} \text{sin}^2(Gx)\text{sec}(Gx)\psi \nonumber \\
    = \frac{-i \text{sin}(Gx)}{G} \text{sec}(Gx) \frac{\partial}{\partial x} \psi + \frac{i}{G} \text{sec}(Gx) G \text{cos}(Gx)\psi + \frac{i \text{sin}(Gx)}{G} \text{sec}(Gx) \frac{\partial}{\partial x} \psi \nonumber \\
    = i \psi; \nonumber \\
    \therefore [\hat{a},\hat{a}^+] = -i[\hat{\chi},\hat{\rho}] = 1
\end{eqnarray}

\begin{figure}
\centering
  \begin{subfigure}{.3\linewidth}
    \centering
    \includegraphics[width = \linewidth]{supplementary_figures/2zeta.png}
    \caption{First image}
  \end{subfigure}%
  \hspace{1em}% Space between image A and B
  \begin{subfigure}{.3\linewidth}
    \centering
    \includegraphics[width = \linewidth]{supplementary_figures/3zeta.png}
    \caption{Second image}
  \end{subfigure}%
  \hspace{2em}% Space between image B and C
  \begin{subfigure}{.3\linewidth}
    \centering
    \includegraphics[width = \linewidth]{supplementary_figures/4zeta.png}
    \caption{Third image}
  \end{subfigure}
  \caption{\label{numorthogonality}
  Inner product of }
\end{figure}

It is useful to state a few more properties explicitly:

\begin{equation}
\label{usefulneelsin} \text{sin}(Gx)|s,n\rangle = G l_{B_0} \left( \sqrt{\frac{n}{2}} |s,n-1\rangle + \sqrt{\frac{n+1}{2}} |s,n+1\rangle\right), 
\end{equation}

\begin{equation}
\label{usefulneelcos} \langle s',n' |\text{cos}(Gx)|s,n\rangle = 0,
\end{equation}

\begin{equation}
\label{usefulneelddx} \frac{\partial}{\partial x} = \left(\frac{G^2 l_{B_0}}{2\sqrt{2}} + \frac{\text{cos}(Gx)}{\sqrt{2}l_{B_0}}\right)\hat{a} + \left(\frac{G^2 l_{B_0}}{2\sqrt{2}} - \frac{\text{cos}(Gx)}{\sqrt{2}l_{B_0}}\right)\hat{a}^+
\end{equation}

\begin{equation}
\label{usefulneelsec} \text{sec}(Gx) \approx \text{cos}^2(Gx)\left(\text{sin}^2(Gx)+1\right)
\end{equation}

Eq. \ref{usefulneelsin} can be shown with a substitution in the argument of the Hermite-gauss basis function, utilizing Eq. \ref{xop}:

\begin{equation}
 G l_{B_0}\frac{\text{sin}(Gx)}{G l_{B_0}}|s,n\rangle = G l_{B_0} |s\rangle \otimes  u \, \Psi_n(u) =  G l_{B_0} \left( \sqrt{\frac{n}{2}} |s,n-1\rangle + \sqrt{\frac{n+1}{2}} |s,n+1\rangle\right), 
\end{equation}

While Eq. \ref{usefulneelcos} can be shown by a shift of the origin to $x = \frac{a_S}{4}$, knowing that the definite integral from -a to a of an odd function will cancel. 

\begin{equation}
\text{typeset this later...}
\end{equation}

Eq.~\ref{usefulneelddx} can be shown either through iterated applications of the chain rule and hermite recursion relation, or through rearrangement of $\hat{\chi}$ and $\hat{\rho}$. Eq.~\ref{usefulneelsec} is instead useful later, where many trig terms will approximate the secant function to fourth order in $\left[\hat{a},\hat{a}^+\right] = 1 - (\frac{1}{\zeta})^4 + ...$ and give rise to the $\rho$ term. We will now project these states onto the Hamiltonian and define the $\tau$ matrices in s-space again. 

\begin{eqnarray}
    \langle s', n', \mathbf{k}|\hat{H}_N| s, n, \mathbf{k}\rangle = -i \eta v_f \langle s', n', \mathbf{k}|\frac{\partial}{\partial y} \sigma_y | s, n, \mathbf{k}\rangle -i \eta v_f \langle s', n', \mathbf{k}|\frac{\partial}{\partial z} \sigma_z | s, n, \mathbf{k}\rangle \nonumber \\ -i \eta v_f \langle s', n', \mathbf{k}|\frac{\partial}{\partial x} \sigma_x | s, n, \mathbf{k}\rangle + 
    \langle s', n', \mathbf{k}| \boldsymbol{\beta}_N\cdot\boldsymbol{\sigma} | s, n, \mathbf{k}\rangle; \\ \nonumber \\
    \label{ddxsxN} -i \eta v_f \langle s', n', \mathbf{k}|\frac{\partial}{\partial y} \sigma_y | s, n, \mathbf{k}\rangle = \frac{\eta v_f k_y}{2}\langle n' |\hbra{s'G^+}{-1}\vket{-i}{-isG^-}|n\rangle \nonumber \\ = \frac{\eta v_f k_y}{2}\langle n' |i\left(-s'G^+ + sG^-\right)|n\rangle = \eta v_f k_y \begin{cases}
          s \langle n'| sin(Gx) |n \rangle   \quad &\text{if} \, s' = s \\
          -i s \langle n'| cos(Gx) |n \rangle \quad &\text{if} \, s' = -s \\
     \end{cases}  \nonumber \\ 
     = \eta v_f k_y s \delta(s'-s)\langle n'|G l_B\left(\sqrt{\frac{n}{2}}|n-1\rangle + \sqrt{\frac{n+1}{2}}|n+1\rangle\right) \nonumber \\ 
     = \eta v_f k_y \tau_z G l_B \left(\sqrt{\frac{n}{2}}\delta(n'-n+1) + \sqrt{\frac{n+1}{2}}\delta(n'-n-1)\right) \\ \nonumber \\
     \label{ddysyN} -i \eta v_f \langle s', n', \mathbf{k}|\frac{\partial}{\partial z} \sigma_z | s, n, \mathbf{k}\rangle =  \frac{\eta v_f k_z}{2} \langle n' |\hbra{s'G^+}{-1}\vket{sG^-}{1}|n\rangle \nonumber \\ = \eta v_f k_z \frac{s's-1}{2}\langle n'|n\rangle = -\eta v_f k_z \tau_x \delta(n'-n)\\
     \langle s', n', \mathbf{k}| \boldsymbol{\beta}_N\cdot\boldsymbol{\sigma} | s, n, \mathbf{k}\rangle = \frac{-J}{2} \langle n'| \hbra{s'G^+}{-1}(G^+\sigma_- +G^-\sigma_+)\vket{sG^-}{-1}|n\rangle = J \langle n'| \hbra{s'G^+}{-1}\vket{G^-}{-s}|n\rangle \label{Jbetasigmaeig}\nonumber \\
     = \frac{J}{2} (s'+s)\langle n'|n\rangle = J \tau_z\delta(n'-n) 
% now for the longitudinal momentum term
\end{eqnarray}
The longitudinal momentum term deserves closer attention: 
\begin{eqnarray}
     -i \eta v_f \langle s', n', \mathbf{k}|\frac{\partial}{\partial x} \sigma_x | s, n, \mathbf{k}\rangle = \frac{-i \eta v_f}{2}\langle n' |\hbra{s'G^+}{-1} \partial_x (\vket{-1}{sG^-}|n\rangle)  \nonumber \\
     = \frac{-i\eta v_f}{2}\langle n'|\hbra{s'G^+}{-1}\left(\vket{0}{-siGG^-}|n\rangle + \vket{-1}{sG^-}\frac{\partial}{\partial x} |n\rangle \right)+ \eta v_f \Xi \nonumber \\ 
    = \frac{\eta v_f G s}{2} \langle n' |e^{-iGx} | n \rangle + \eta v_f \Xi + \eta v_f \begin{cases}
          -i s \langle n'| \text{cos} (Gx) \frac{\partial}{\partial x } |n\rangle    \quad &\text{if} \, s' = s \\
          s \langle n'| \text{sin}(Gx) \frac{\partial}{\partial x } |n\rangle  \quad &\text{if} \, s' = -s \\
     \end{cases}  \nonumber \\
\end{eqnarray}

The first term can be decomposed using euler's identity, then evaluated using identities Eq.~\ref{usefulneelsin} and Eq.~\ref{usefulneelcos}:

\begin{eqnarray}
    \frac{\eta v_f G s}{2} \langle n'| e^{-iGx} | n\rangle = \frac{\eta v_f G s}{2} \langle n'| \left(\text{cos}(Gx) - i \text{sin}(Gx) \right)| n\rangle  = 0 + \frac{-i \eta v_f G s}{2} \langle n'| \left(\text{sin}(Gx) \right)| n\rangle  \nonumber \\
    = \frac{-i \eta v_f G^2 l_{B_0} s}{2} \langle n'|\left(\sqrt{\frac{n}{2}}|n-1\rangle + \sqrt{\frac{n+1}{2}}|n+1\rangle \right) \nonumber \\
    \frac{\eta v_f G^2 l_{B_0} }{2} (\tau_y + i \tau_z) \left(\sqrt{\frac{n}{2}}\delta(n'-n+1)+\sqrt{\frac{n+1}{2}}\delta(n'-n-1)\right). 
\end{eqnarray}

The third term can be evaluated by concatenating the aforementioned identities, along with Eq.~\ref{usefulneelddx}. The trigonometric identity $\text{cos}^2(Gx) = 1 - \text{sin}^2(Gx)$ is also used, and the higher states of order $\zeta^{-2}$ are discarded.
\begin{eqnarray}
% trig ish identity
\langle n' | \text{sin}(Gx) \text{cos}(Gx) |n\rangle = \langle n' | \text{cos}(Gx) \left(\sqrt{\frac{n}{2}}|n-1\rangle+\sqrt{\frac{n+1}{2}}|n+1\rangle \right) = 0; \\ 
% higher order sin terms
\langle n' | \text{cos}^2(Gx) |n\rangle = \langle n' | n\rangle + G l_{B_0} \langle n' | \text{sin}(Gx) \left(\sqrt{\frac{n}{2}}|n-1\rangle+\sqrt{\frac{n+1}{2}}|n+1\rangle \right) \nonumber \\
= \delta_{n',n} + \frac{(G l_{B_0})^2}{2}\langle n' |\left(\sqrt{n(n-1)}|n-2\rangle+(2n+1)|n\rangle +\sqrt{(n+2)(n+1)}|n+2\rangle \right) \nonumber \\
\equiv \hat{I}_n + \frac{1}{2\zeta^2}\left(a^+a^+ + a^+a + aa^+ + aa \right); \\
% useful true thing about derivative operator
\frac{\partial}{\partial x}|n\rangle  = \left(\frac{G^2 l_{B_0}}{2} + \frac{\text{cos}(Gx)}{l_{B_0}}\right)\sqrt{\frac{n}{2}}|n-1\rangle + \left(\frac{G^2 l_{B_0}}{2} - \frac{\text{cos}(Gx)}{l_{B_0}}\right)\sqrt{\frac{n+1}{2}}|n+1\rangle; \\
% useful true thing about derivative operator prepending with sin(Gx)
\langle n'|\text{sin}(Gx)\frac{\partial}{\partial x}|n\rangle  = \langle n' | \text{sin}(Gx) \left[\left(\frac{G^2 l_{B_0}}{2} + \frac{\text{cos}(Gx)}{l_{B_0}}\right)\sqrt{\frac{n}{2}}|n-1\rangle + \left(\frac{G^2 l_{B_0}}{2} - \frac{\text{cos}(Gx)}{l_{B_0}}\right)\sqrt{\frac{n+1}{2}}|n+1\rangle\right] \nonumber \\
=  G \frac{(G l_{B_0})^2}{4} \langle n' |\left(\sqrt{n(n-1)}|n-2\rangle+(2n+1)|n\rangle +\sqrt{(n+2)(n+1)}|n+2\rangle \right) \nonumber \\
\equiv \frac{G}{4\zeta^2}\left(a^+a^+ + a^+a + aa^+ + aa \right);\\
% final expression of this subterm
\eta v_f\begin{cases}
          -i s \langle n'| \text{cos}(Gx) \left[\left(\frac{G^2 l_{B_0}}{2} + \frac{\text{cos}(Gx)}{l_{B_0}}\right)\sqrt{\frac{n}{2}}|n-1\rangle + \left(\frac{G^2 l_{B_0}}{2} - \frac{\text{cos}(Gx)}{l_{B_0}}\right)\sqrt{\frac{n+1}{2}}|n+1\rangle \right]   \quad &\text{if} \, s' = s \\
          s \langle n'| \text{sin}(Gx) \left[\left(\frac{G^2 l_{B_0}}{2} + \frac{\text{cos}(Gx)}{l_{B_0}}\right)\sqrt{\frac{n}{2}}|n-1\rangle + \left(\frac{G^2 l_{B_0}}{2} - \frac{\text{cos}(Gx)}{l_{B_0}}\right)\sqrt{\frac{n+1}{2}}|n+1\rangle \right] \quad &\text{if} \, s' = -s \\
     \end{cases} \nonumber \\ 
     \approx \frac{\eta v_f }{l_{B_0}} i \tau_z \left(\sqrt{\frac{n}{2}}\delta(n'-n+1) - \sqrt{\frac{n+1}{2}}\delta(n'-n-1)\right)
\end{eqnarray}

Finally, the second term warrants a treatment akin to the phase slips of the Bloch helix case... working on it.
