# Supplementary material for: Flat bands and multi-state memory devices from chiral domain wall superlattices in magnetic Weyl semimetals
Source: arXiv:2303.16918 source file (2023-10-23)
Supplement: Supplementary file 2 [file supplementary3.tex]

\subsection{Ladder operators for Neel and Bloch exchange helix Hamiltonians}

First, start off with the Hermite-Gauss functions $\Psi_n(u)$, with recursion relations:

\begin{eqnarray}
 \label{xop} u|n\rangle = \frac{1}{\sqrt{2}}\left(\sqrt{n}|n-1\rangle + \sqrt{n+1}|n+1\rangle\right) \\
\frac{\partial}{\partial u} |n\rangle = \frac{1}{\sqrt{2}}\left(\sqrt{n}|n-1\rangle - \sqrt{n+1}|n+1\rangle \right)
\end{eqnarray}

Then, we can modify the arguments to fit to each problem. For the Bloch and Neel helix cases respectively, let 
\begin{equation}
u_B = \frac{e^{iGx}}{G l_B},
\end{equation}
\begin{equation}
u_N = \frac{\text{sin}(Gx)}{G l_B}.
\end{equation}

Through a previous setup as in the Neel DW hamiltonian, we can define a prefactor on these basis states such that they are orthonormal for large enough $\zeta = (Gl_B)^{-1}$ or small enough n:

\begin{equation}
\Psi_{n,B} = \sqrt{\frac{e^{iGx}}{l_B}}\Psi_n\left(\frac{e^{iGx}}{G l_B}\right)
\end{equation}

\begin{equation}
\Psi_{n,N} = \sqrt{\frac{|cos(Gx)|}{l_B}}\Psi_n\left(\frac{sin(Gx)}{G l_B}\right)
\end{equation}

It can be shown through u-substitution or through the numerical plots on page 15 that these states are nearly orthonormal. Let us now construct a set of ladder operators which act on these states. The position-like operator is intuitive for both:

\begin{equation}
\hat{\chi}_B = \frac{e^{iGx}}{G l_B}; \; \; \hat{\chi}_N = \frac{\text{sin}(Gx)}{G l_B}.
\end{equation}

While the momentum-like operator can be defined such that $[a,a^+] = 1$

\begin{align*}
    \hat{\rho}_B = -l_B e^{-iGx} \frac{\partial}{\partial x} \\
    \hat{\rho}_N = -i l_{B_0} \text{sec}(Gx) \frac{\partial}{\partial x} + i \frac{G l_{B_0}}{2}\text{sec}(Gx)\text{sin}(Gx);\\
    \hat{a} = \frac{1}{\sqrt{2}}\left(\hat{\chi} + i \hat{\rho}\right); \; \; \hat{a}^+ = \frac{1}{\sqrt{2}}\left(\hat{\chi}^+ - i \hat{\rho}^+\right)
\end{align*}

We can show the commutation relation for the Bloch, then Neel wall cases:
\begin{eqnarray}
    [\hat{a},\hat{a}^+] = \frac{1}{2}\left(\hat{\chi}^2 + \hat{\rho}^2 -i[\hat{\chi},\hat{\rho}] - \left(\hat{\chi}^2 + \hat{\rho}^2 +i[\hat{\chi},\hat{\rho}]\right)\right) \nonumber \\
    = -i[\hat{\chi},\hat{\rho}]; \nonumber \\
    %bloch dw conjugate variable commutation
    \left[\hat{\chi}_B,\hat{\rho}_B\right]\psi = \frac{-e^{iGx}}{G} e^{-iGx} \frac{\partial}{\partial x} \psi  + e^{-iGx} \frac{\partial}{\partial x} \left(\frac{-e^{iGx}}{G}\psi\right)   \nonumber \\
    = \frac{-1}{G} \frac{\partial}{\partial x} \psi  + \frac{1}{G} \frac{\partial}{\partial x} + i \psi \nonumber \\
    = i \psi; \nonumber \\
    \therefore [\hat{a}_B,\hat{a}^+_B] = -i[\hat{\chi}_B,\hat{\rho}_B] = 1 \\ 
    % now show for Neel helix case
    \left[\hat{\chi}_N,\hat{\rho}_N\right]\psi = \frac{-i \text{sin}(Gx)}{G} \text{sec}(Gx) \frac{\partial}{\partial x} \psi + \frac{i}{2} \text{sin}^2(Gx)\text{sec}(Gx)\psi \nonumber \\
    + \frac{i}{G} \text{sec}(Gx) \frac{\partial}{\partial x} \left(\text{sin}(Gx) \psi\right) -\frac{i}{2} \text{sin}^2(Gx)\text{sec}(Gx)\psi \nonumber \\
    = \frac{-i \text{sin}(Gx)}{G} \text{sec}(Gx) \frac{\partial}{\partial x} \psi + \frac{i}{G} \text{sec}(Gx) G \text{cos}(Gx)\psi + \frac{i \text{sin}(Gx)}{G} \text{sec}(Gx) \frac{\partial}{\partial x} \psi \nonumber \\
    = i \psi; \nonumber \\
    \therefore [\hat{a}_N,\hat{a}^+_N] = -i[\hat{\chi}_N,\hat{\rho}_N] = 1
\end{eqnarray}

While the $\text{sec}(Gx)$ term of $\hat{\rho}_N$ is perhaps unphysical, a good approximation to $\text{sec}(Gx)$ could come up when projecting the exchange term spinor wavefunctions onto $H_N$:

\begin{equation}
\text{cos}(Gx)\left(\text{sin}^2(Gx) + 1\right) \approx \text{sec}(Gx)
\end{equation}

Supposing the states are locally like the H.O. eigenfunctions, which is true for these wavefunctions, then $[a,a^+] = 1 - \zeta^{-4} + ...$ when taylor expanding around one of these sites. A much worse approximation to $\text{sec}(Gx)$ is 

\begin{equation}
\text{cos}(Gx) \approx \text{sec}(Gx)
\end{equation}

Which I suspect will have leading-order corrections of order $[a,a^+] = 1 - \zeta^{-2} + ...$, though I have not worked through the math... I do know, however, that such prefactors on $\frac{\partial}{\partial x  }$ explictly come up in the Hamiltonian during a change of basis.  

I have been working to express the hamiltonians in terms of these operators with moderate success. I am optimistic about this, as the exchange terms for the Bloch wall case are explicitly just  $\chi_B$, and the kinetic energy terms transform into something like $\rho_B$ after basis transformation by projection onto the exchange term eigenspinors. For the Neel wall case, after gauging away the $\sigma_x$ term, the same is true for $\chi_N$. Also, the wavefunctions for $\Psi_B$ and $\Psi_N$ both have intuitive properties that make a lot of sense, if we take them to be the superlattice-periodic part of the bloch functions.
